# Supplementary material for: Strain engineered higher order topological phases for spin-3/2 Luttinger fermions
Source: arXiv:1907.12568 source file (2020-03-02)
Supplement: Supplementary file 1 [file NematicHOT_Supplementary.pdf]

# Supplementary Material: Strain engineered higher order topological phases for spin-3/2 Luttinger fermions

András L. Szabó,[1] Roderich Moessner,[1] and Bitan Roy[1]

[1]*Max-Planck-Institut für Physik komplexer Systeme, Nöthnitzer Str. 38, 01187 Dresden, Germany*

(Dated: July 29, 2019)

The Supplementary Material contains: (1) representation of five mutually anticommuting four-component Γ matrices as symmetric traceless tensor operators formed from bilinear products of spin-3/2 matrices, (2) transformation of Luttinger Hamiltonian in the presence of external strain applied along the $y$ axis and along the $\langle 111 \rangle$ directions, (3) boundary modes of three dimensional first and second order Dirac semimetals and topological insulators of spin-1/2 fermions, and (4) block-diagonal form of the Luttinger Hamiltonian for spin-3/2 fermions in the $k_z = 0$ plane.

## I. REPRESENTATION OF Γ MATRICES IN TERMS OF SPIN-3/2 MATRICES

Five mutually anticommuting Γ matrices appearing in the Luttinger Hamiltonian $\hat{h}_{\rm L}(\mathbf{k})$, see Eq. (3) of the main paper, can be constructed from the spin-3/2 matrices according to [1]

$$\Gamma_1 = \frac{1}{\sqrt{3}}\,\{S_y, S_z\},\;\; \Gamma_2 = \frac{1}{\sqrt{3}}\,\{S_z, S_x\},\;\; \Gamma_3 = \frac{1}{\sqrt{3}}\,\{S_x, S_y\},\;\; \Gamma_4 = \frac{1}{\sqrt{3}}\,(S_x^2 - S_y^2),\;\; \Gamma_5 = \frac{1}{2}(2S_z^2 - S_x^2 - S_y^2). \tag{1}$$

Here $\{A, B\} = AB + BA$ is the anticommutator. The above five Γ matrices are the components of the rank-two symmetric traceless tensor operator [2]

$$T_{\mu\nu} = \frac{1}{\sqrt{3}}\left[\{S_\mu, S_\nu\} - \frac{2}{3}\delta_{\mu\nu}\,\boldsymbol{S}^2\right], \tag{2}$$

which transforms in the $S = 2$ representation of $SU(2)$ under spin rotations. In the basis specified in the main text, the spin-3/2 matrices are defined as

$$S_x = \frac{1}{2}\begin{bmatrix} 0 & \sqrt{3} & 0 & 0 \\ \sqrt{3} & 0 & 2 & 0 \\ 0 & 2 & 0 & \sqrt{3} \\ 0 & 0 & \sqrt{3} & 0 \end{bmatrix}, \quad S_y = \frac{i}{2}\begin{bmatrix} 0 & -\sqrt{3} & 0 & 0 \\ \sqrt{3} & 0 & -2 & 0 \\ 0 & 2 & 0 & -\sqrt{3} \\ 0 & 0 & \sqrt{3} & 0 \end{bmatrix}, \quad S_z = \frac{1}{2}\begin{bmatrix} 3 & 0 & 0 & 0 \\ 0 & 1 & 0 & 0 \\ 0 & 0 & -1 & 0 \\ 0 & 0 & 0 & -3 \end{bmatrix}. \tag{3}$$

## II. EFFECTS OF EXTERNAL STRAIN ALONG $y$ AXIS AND $\langle 111 \rangle$ DIRECTIONS

In the main text, we address the effects of $E_g$ strain applied along the $z$ and $x$ axes. Here, we present some key details of analogous analysis, when the strain is applied along the $y$ axis, for which we introduce a new set of momentum $q_x = k_x$, $q_y = k_z$, $q_z = k_y$, such that $q_z \parallel [010]$. Accordingly, we introduce a new set of mutually anticommuting $\bar{\Gamma}$ matrices, satisfying the anitcommuting Clifford algebra $\{\bar{\Gamma}_j, \bar{\Gamma}_k\} = 2\delta_{jk}$ for $j, k = 1, \cdots, 5$

$$\bar{\Gamma}_1 = \Gamma_1,\; \bar{\Gamma}_2 = \Gamma_3,\; \bar{\Gamma}_3 = \Gamma_2,\; \bar{\Gamma}_4 = \frac{1}{2}(\Gamma_4 - \sqrt{3}\Gamma_5),\; \bar{\Gamma}_5 = -\frac{1}{2}(\sqrt{3}\Gamma_4 + \Gamma_5).$$

Under these transformations, the effective single particle Hamiltonian reads [see Eqs. (3) and (5) of the main text]

$$\hat{h}_{\rm L}(\mathbf{k}) + \hat{h}^y_{E_g} = -\frac{1}{2m}\sum_{j=1}^{5} d_j(\mathbf{k})\Gamma_j - \frac{|\Delta|}{2}\left[\sqrt{3}\,\Gamma_4 + \Gamma_5\right]\,{\rm sgn}(\Delta) \equiv -\frac{1}{2m}\sum_{j=1}^{5} d_j(\mathbf{q})\bar{\Gamma}_j + |\Delta|\,{\rm sgn}(\Delta)\bar{\Gamma}_5, \tag{4}$$

which takes the form of Eq. (6) of the main text (obtained when strain is applied along the [001] direction).

In the main text, we also addressed the effects of external strain applied along one of the specific $\langle 111 \rangle$ or $C_{3v}$ or body diagonal directions (the $T_{2g}$ strain), namely the [111] direction. We here display the key steps of the analogous

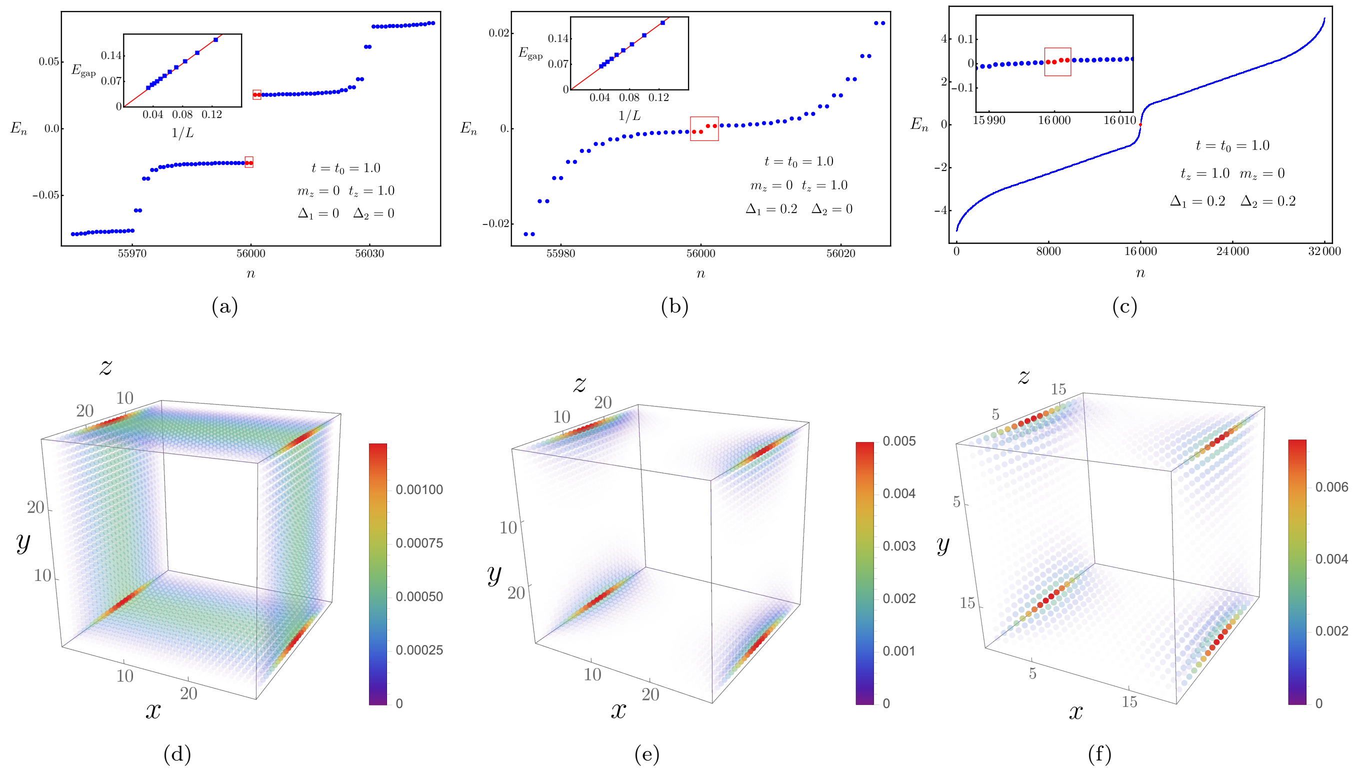


Figure 1: Energy spectra of first [second] order Dirac semimetals are shown in (a) [(b) and (c)]. Here, $n$ is the index of energy eigenvalue $E_n$. Various parameters, appearing in Eqs. (8) and (9), for the numerical simulation are shown in each panel. We diagonalize the tight binding model on a cubic lattice of linear dimension $L$ in all directions, where $L = 30$ for (a) and (b), and $L = 20$ for (c). The finite spectral gaps ($E_{gap}$) near zero energy in panels (a) and (b) are solely due to finite system effects, which vanish as $L \to \infty$ (see insets). A similar gap also exists among four states (marked in red) in panel (c), which also vanishes as $L \to \infty$ (not shown here explicitly). Hence, the system always describes a Dirac semimetal in the thermodynamic limit ($L \to \infty$). (d) Local density of states (LDoS) associated with the Fermi arc surface states [see red dots in (a)], occupying the two dimensional $xz$ and $yz$ surfaces (thus characterized by codimension $d_c = 1$). LDoS associated with four hinge modes of $d_c = 2$ appearing in panels (b) and (c) are respectively shown in (e) and (f). For finite $\Delta_2$ the energy spectra lose spectral symmetry about zero energy, but we continue to find four hinge modes at half-filling.

analysis, when the strain is applied along the other three body diagonals. First, we consider the strain applied along the $[1\bar{1}\bar{1}]$ direction. Then $\text{sgn}(\Delta_1) = +(-)$, $\text{sgn}(\Delta_2) = -(+)$ and $\text{sgn}(\Delta_3) = -(+)$ for tensile (compressive) strain, yielding $\text{sgn}(\Delta) = +(-)$ [see Eq. (9) of the main text]. We now introduce the following set of momenta

$$q_x = \frac{k_x + k_y}{\sqrt{2}}, \; q_y = \frac{k_x - k_y + 2k_z}{\sqrt{6}}, \; q_z = \frac{k_x - k_y - k_z}{\sqrt{3}},$$

such that $q_z \parallel [1\bar{1}\bar{1}]$, and a set of five mutually anticommuting $\bar{\Gamma}$ matrices

$$\begin{aligned} \bar{\Gamma}_1 &= -\left[\frac{1}{3\sqrt{2}}\left(\Gamma_1 - \Gamma_2 + 2\Gamma_3\right) + \sqrt{\frac{2}{3}}\,\Gamma_5\right], \; \bar{\Gamma}_2 = -\frac{\Gamma_1 + \Gamma_2 - 2\Gamma_4}{\sqrt{6}}, \; \bar{\Gamma}_3 = \frac{\Gamma_1 + \Gamma_2 + \Gamma_4}{\sqrt{3}}, \\ \bar{\Gamma}_4 &= \frac{\Gamma_1 - \Gamma_2 + 2\Gamma_3 - \sqrt{3}\Gamma_5}{3}, \; \bar{\Gamma}_5 = \frac{\Gamma_1 - \Gamma_2 - \Gamma_3}{\sqrt{3}}, \end{aligned}$$

such that they satisfy the anitcommuting Clifford algebra $\{\bar{\Gamma}_j, \bar{\Gamma}_k\} = 2\delta_{jk}$ for $j,k = 1, \cdots, 5$. Then the effective single particle Hamiltonian reads

$$\hat{h}_{\rm L}(\mathbf{k}) + \frac{|\Delta|}{\sqrt{3}}\left[\Gamma_1 - \Gamma_2 - \Gamma_3\right]\,\text{sgn}(\Delta) \equiv -\frac{1}{2m}\sum_{j=1}^{5} d_j(\mathbf{q})\bar{\Gamma}_j + |\Delta|\,\bar{\Gamma}_5\,\text{sgn}(\Delta), \tag{5}$$

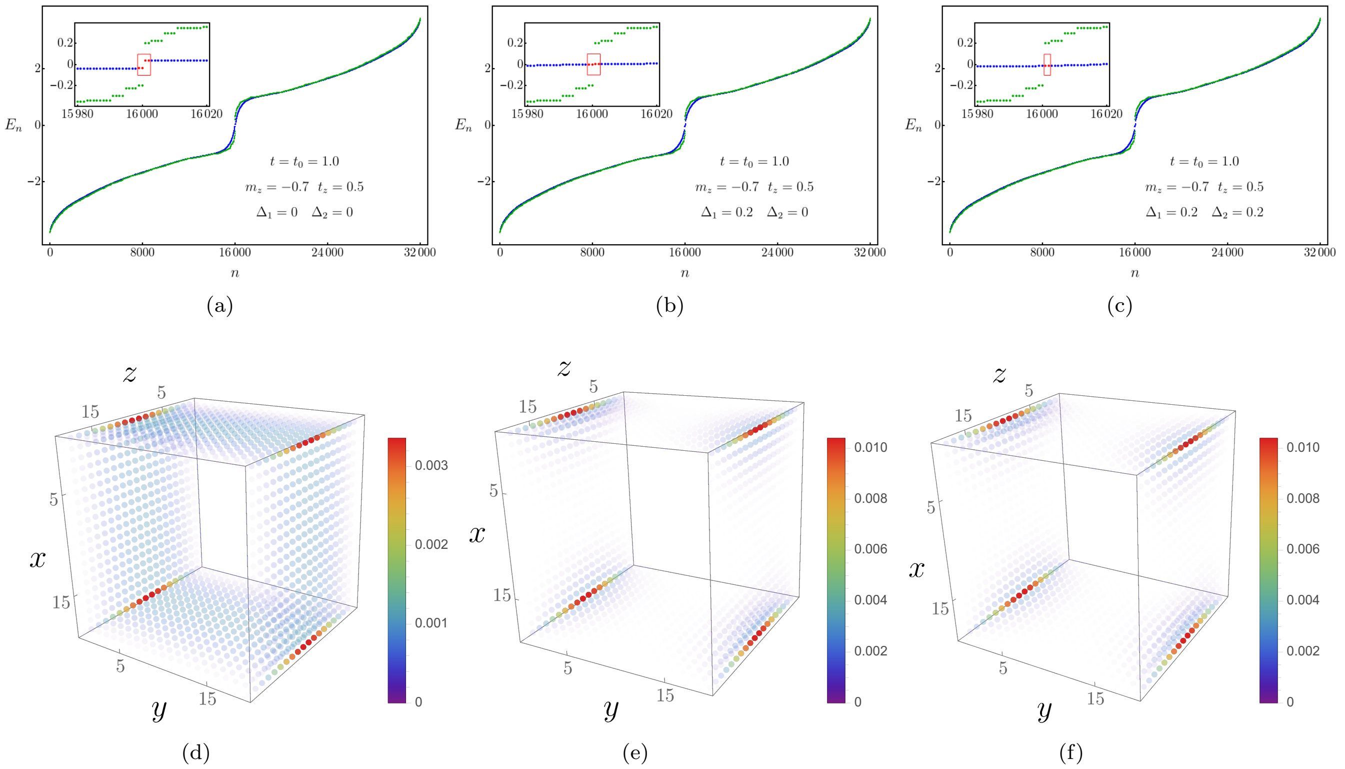


Figure 2: Energy spectra of first [second] order topological insulators are shown in (a) [(b) and (c)] with periodic (green) and open (blue) boundaries. Here, $n$ is the index of energy eigenvalue $E_n$. Various parameters appearing in Eqs. (8) and (9), for the numerical simulation are shown in each panel. We diagonalize the tight binding model on a cubic lattice of linear dimension $L = 20$ in all directions. (d) Local density of states (LDoS) associated with the Fermi arc surface states [see red dots in (a)], occupying the two dimensional $xz$ and $yz$ surfaces (thus characterized by codimension $d_c = 1$). LDoS associated with four hinge modes of $d_c = 2$, appearing in panels (b) and (c) [see the red dots] are shown in (e) and (f). For finite $\Delta_2$ the energy spectra lose spectral symmetry about zero energy, but we continue to find four hinge modes at half-filling.

which takes the form of Eq. (6) of the main text.

Next we assume the $T_{2g}$ strain applied along the $[\bar{1}1\bar{1}]$ direction, such that tensile (compressive) strain corresponds to $\text{sgn}(\Delta_1) = -(+)$, $\text{sgn}(\Delta_2) = +(-)$ and $\text{sgn}(\Delta_3) = -(+)$, yielding $\text{sgn}(\Delta) = +(-)$ [see Eq. (9) of the main text]. We introduce the following set of momenta

$$q_x = \frac{k_x + k_y}{\sqrt{2}}, \;\; q_y = \frac{k_x - k_y - 2k_z}{\sqrt{6}}, \;\; q_z = \frac{-k_x + k_y - k_z}{\sqrt{3}},$$

such that $q_z \parallel [\bar{1}1\bar{1}]$ and a new set of mutually anticommuting $\bar{\Gamma}$ matrices according to

$$\begin{aligned} \bar{\Gamma}_1 &= -\left[\frac{1}{3\sqrt{2}}\left(\Gamma_1 - \Gamma_2 - 2\Gamma_3\right) - \sqrt{\frac{2}{3}}\,\Gamma_5\right], \;\; \bar{\Gamma}_2 = -\frac{\Gamma_1 + \Gamma_2 + 2\Gamma_4}{\sqrt{6}}, \;\; \bar{\Gamma}_3 = \frac{-\Gamma_1 - \Gamma_2 + \Gamma_4}{\sqrt{3}}, \\ \bar{\Gamma}_4 &= \frac{\Gamma_1 - \Gamma_2 - 2\Gamma_3 + \sqrt{3}\Gamma_5}{3}, \;\; \bar{\Gamma}_5 = \frac{-\Gamma_1 + \Gamma_2 - \Gamma_3}{\sqrt{3}}, \end{aligned}$$

such that they satisfy the anitcommuting Clifford algebra $\{\bar{\Gamma}_j, \bar{\Gamma}_k\} = 2\delta_{jk}$ for $j, k = 1, \cdots, 5$. Then the effective single particle Hamiltonian reads

$$\hat{h}_{\rm L}(\mathbf{k}) + \frac{|\Delta|}{\sqrt{3}}\left[-\Gamma_1 + \Gamma_2 - \Gamma_3\right]\, \text{sgn}(\Delta) \equiv -\frac{1}{2m}\sum_{j=1}^{5} d_j(\mathbf{q})\bar{\Gamma}_j + |\Delta|\,\bar{\Gamma}_5\, \text{sgn}(\Delta), \qquad (6)$$

which takes the form of Eq. (6) of the main text.

Finally, we consider the $T_{2g}$ strain applied along the $[\bar{1}\bar{1}1]$ direction, such that tensile (compressive) strain corresponds to $\text{sgn}(\Delta_1) = -(+)$, $\text{sgn}(\Delta_2) = -(+)$ and $\text{sgn}(\Delta_3) = +(-)$, yielding $\text{sgn}(\Delta) = +(-)$ [see Eq. (9) of the main text]. We introduce the following set of momenta

$$q_x = \frac{k_x - k_y}{\sqrt{2}}, \; q_y = \frac{k_x + k_y + 2k_z}{\sqrt{6}}, \; q_z = \frac{-k_x - k_y + k_z}{\sqrt{3}},$$

such that $q_z \parallel [\bar{1}\bar{1}1]$ and a new set of mutually anticommuting $\bar{\Gamma}$ matrices according to

$$\bar{\Gamma}_1 = -\left[\frac{1}{3\sqrt{2}}\left(\Gamma_1 + \Gamma_2 + 2\Gamma_3\right) - \sqrt{\frac{2}{3}}\,\Gamma_5\right], \; \bar{\Gamma}_2 = -\frac{\Gamma_1 - \Gamma_2 + 2\Gamma_4}{\sqrt{6}}, \; \bar{\Gamma}_3 = \frac{-\Gamma_1 + \Gamma_2 + \Gamma_4}{\sqrt{3}},$$

$$\bar{\Gamma}_4 = \frac{\Gamma_1 + \Gamma_2 + 2\Gamma_3 + \sqrt{3}\Gamma_5}{3}, \; \bar{\Gamma}_5 = \frac{-\Gamma_1 - \Gamma_2 + \Gamma_3}{\sqrt{3}},$$

such that they satisfy the anitcommuting Clifford algebra $\{\bar{\Gamma}_j, \bar{\Gamma}_k\} = 2\delta_{jk}$ for $j,k = 1, \cdots, 5$. Then the effective single particle Hamiltonian reads

$$\hat{h}_{\rm L}(\mathbf{k}) + \frac{|\Delta|}{\sqrt{3}}\left[-\Gamma_1 - \Gamma_2 + \Gamma_3\right] \, \text{sgn}(\Delta) \equiv -\frac{1}{2m}\sum_{j=1}^{5} d_j(\mathbf{q})\bar{\Gamma}_j + |\Delta| \, \bar{\Gamma}_5 \, \text{sgn}(\Delta), \tag{7}$$

which again takes the form of Eq. (6) of the main text.

Therefore, when the external strain is applied along any high symmetry $\langle 001\rangle$ or $\langle 111\rangle$ directions, the effective single particle Hamiltonian can always be cast in the form of $\hat{h}^{z,t}_{E_g}$ [see Eq. (6) of the main text], capturing the effects of an external strain applied along the $z$ or [001] direction. Therefore, analysis of the emergent topology from $\hat{h}^{z,t}_{E_g}$ [see main text] is sufficient to address the effects of external strian, applied along any high symmetry direction.

## III. HIGHER ORDER TOPOLOGICAL PHASES OF SPIN-1/2 FERMIONS

A tight binding model describing a three-dimensional topological Dirac semimetal or insulator is given by

$$\hat{h}^{\mathbf{k}}_0 = t\sum_{j=1}^{2} \sin(k_j a)\,\gamma_j + \left[t_z\cos(k_z a) - m_z + t_0\sum_{j=1}^{2}\left[1-\cos(k_j a)\right]\right]\gamma_3, \tag{8}$$

where $a$ is the lattice spacing, set to be unity, and $\gamma_j$s define a set of mutually anticommuting four-component Hermitian matrices, satisfying $\{\gamma_j, \gamma_k\} = 2\delta_{jk}$ for $j,k = 1, \cdots, 5$. The outcomes, summarized in Figs. 1 and 2, do not depend on the representation of the $\gamma$ matrices. Nonetheless, for the sake of concreteness we commit to a specific representation in which $\gamma_1 = \sigma_3\tau_1$, $\gamma_2 = \sigma_0\tau_2$, $\gamma_3 = \sigma_0\tau_3$, $\gamma_4 = \sigma_1\tau_1$ and $\gamma_5 = \sigma_2\tau_1$. Two sets of Pauli matrices $\boldsymbol{\sigma}$ and $\boldsymbol{\tau}$ respectively operate on spin and sublattice/orbital indices. We diagonalize the above Hamiltonian on a cubic lattice. The global phase diagram of the above model displays a confluence of topological (gapless as well as gapped) and trivial phases, which has been discussed in details in Ref. [3]. Instead of delving into such discussion again, we here focus on a few specific and relevant cases. For example, a three-dimensional topological Dirac semimetal is realized for $t = t_z = t_0 = 1$ and $m = 0$, and the Dirac points are then located at $(0, 0, \pm\pi/2)$. This phase supports doubly degenerate Fermi arc surface states [see Fig. 1(a)] that occupy the two-dimensional $xz$ and $yz$ surfaces, see Fig. 1(e). On the other hand, a three-dimensional topological quantum spin Hall insulator is found for $t = t_0 = 1$, $t_z = 0.5$ and $m_z = -0.7$, for example. This phase also supports two-dimensional Fermi arc surface states, as shown in Figs. 2(a) and 2(e). Therefore, the Fermi arcs are characterized by codimension $d_c = 1$, and these two topological phases are first order. Finally, we note that since $\hat{h}^{\mathbf{k}}_0$ contains only three mutually anticommuting matrices, it can always be cast into a block diagonal form and each such block is two-dimensional. Hence, $\hat{h}^{\mathbf{k}}_0$ is described by effective spin-1/2 fermions.

Second order topological phases can now be constructed by systematically reducing the dimensionality of Fermi arc surface states. This can be achieved by adding the following four-fold symmetry breaking perturbations

$$\hat{h}_1^{\mathbf{k}} = \Delta_1 \; [\cos(k_y a) - \cos(k_x a)] \; \gamma_4 + \Delta_2 \; \sin(k_x a) \sin(k_y a) \; \gamma_5. \tag{9}$$

Since $\{\hat{h}_0^{\mathbf{k}}, \hat{h}_1^{\mathbf{k}}\} = 0$, the above two perturbations act as masses for the two dimensional Fermi arc surface states. However, both of them change sign under four-fold or $C_4$ rotation, and hence the Fermi arcs get only partially gapped in their presence, yielding one-dimensional hinge modes with $d_c = 2$. The system then describes second order topological phases. The underlying mechanism of such systematic dimensional reduction of the topological surface states is discussed in the main text. Numerical demonstration of the hinge modes for a second order Dirac semimetal and topological insulator are respectively shown in Figs. 1 and 2.

## IV. LUTTINGER HAMILTONIAN IN THE $k_z = 0$ PLANE

The Luttinger Hamiltonian in the presence of an external strain in the $z$ direction and on the $k_z = 0$ plane reads

$$\hat{h}^{z,t}_{E_g}(k_z = 0) = \left[ |\Delta| \mathrm{sgn}(\Delta) + \frac{k_\perp^2}{4m} \right] \Gamma_5 - \frac{1}{2m} \left[ d_3(\mathbf{k}) \Gamma_3 + d_4(\mathbf{k}) \Gamma_4 \right]. \tag{10}$$

Recall that $\Gamma_3 = \kappa_2 \sigma_0$, $\Gamma_4 = \kappa_1 \sigma_0$ and $\Gamma_5 = \kappa_3 \sigma_3$. Since the above Hamiltonian involves only three mutually anticommuting matrices, it can be cast in the block diagonal form, where each block is two-dimensional. This can be accomplished by arranging the four-component spinor basis according to $\Psi^\top_{\mathbf{k}} = (c_{\mathbf{k},\frac{3}{2}}, c_{\mathbf{k},-\frac{1}{2}}, c_{\mathbf{k},\frac{1}{2}}, c_{\mathbf{k},-\frac{3}{2}})$. Then we find $\hat{h}^{z,t}_{E_g}(k_z = 0) = H_+ \oplus H_-$, where for $\sigma = \pm$

$$H_\sigma = \left[ |\Delta| \; \mathrm{sgn}(\Delta) + \frac{k_\perp^2}{4m} \right] \sigma \tau_3 - \frac{1}{2m} \left[ d_4(\mathbf{k}) \tau_1 + d_3(\mathbf{k}) \tau_2 \right], \tag{11}$$

identical to Eq. (7) of the main text.

[1] S. Murakami, S-C. Zhang, and N. Nagaosa, Phys. Rev. B **69**, 235206 (2004).
[2] B. Roy, S. A. A. Ghorashi, M. S. Foster and A. H. Nevidomskyy, Phys. Rev. B **99**, 054505 (2019).
[3] B. Roy, R-J. Slager and V. Juričić, Phys. Rev. X **8**, 031076 (2018).
